# Supplementary material for: Delayed feedback causes non-Markovian behavior of neuronal firing statistics
Source: arXiv:1012.6019 ancillary file (2010-12-30)
Supplement: Supplementary file 1 [file movie.pdf]

**Kravchuk K.G. and Vidybida A.K.**

# Delayed feedback causes non-Markovian behavior of neuronal firing statistics

supplementary material
use adobe acrobat to see animation

**Journal of Physics A**

run time: 1 ms

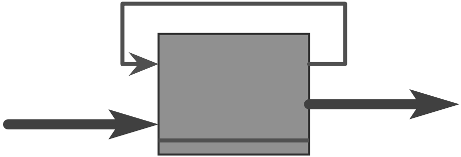

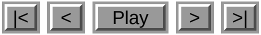


Binding neuron with feedback in action

Neuron is fed with Poisson stream of intensity $\lambda = 0.05$ ms$^{-1}$.
Internal memory $\tau = 20$ ms. Threshold $N_0 = 2$.
Delay in the feedback line $\Delta = 19$ ms.

run time: 1 ms

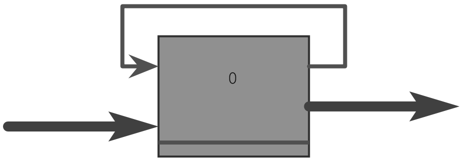


|< < Play > >|

Binding neuron with feedback in action

Neuron is fed with Poisson stream of intensity $\lambda = 0.135\ \mathrm{ms}^{-1}$.
Internal memory $\tau = 20$ ms. Threshold $N_0 = 4$.
Delay in the feedback line $\Delta = 22$ ms.

Credits

Prepared with animfig package by Kevin Pulo

`http://www.cs.usyd.edu.au/~kev/animfig/`
